# Supplementary material for: Melding Wildlife Surveys to Improve Conservation Inference
Source: arXiv:2211.12642 source file (2023-04-12)
Supplement: Supplementary file 1 [file LEPC_IM_appendix.pdf]

# Web Appendix: Melding Wildlife Surveys to Improve Conservation Inference.

## A MODEL STATEMENTS

### A.1 AERIAL DISTANCE SAMPLING SUBMODEL

$$\begin{aligned}
 v_{itl} &\sim \text{Binomial}(B_{itl}, \rho_{itl}) \\
 B_{itl} &= \begin{cases} 2, & \text{for } d_{itl} > 7, \epsilon_{itl} = 1, \text{ and } z_{itl} = 1 \\ 1, & \text{for } d_{itl} > 7, \epsilon_{itl} = 0, \text{ and } z_{itl} = 1 \\ 1, & \text{for } d_{itl} \leq 7 \text{ and } z_{itl} = 1 \\ 0, & \text{for } z_{itl} = 0 \end{cases}, \\
 \text{logit}(\boldsymbol{\rho}) &= (\mathbf{X}_\rho, \mathbf{N}, \mathbf{d}) \boldsymbol{\beta}_\rho, \boldsymbol{\beta}_\rho \sim \mathcal{N}(\mathbf{0}, 2.25\mathbf{I}), \\
 N_{itl} &\sim \begin{cases} \text{ZTP}(\lambda_{it}), & \text{for } \omega_{itl} = 1 \\ \text{ZTP}(\lambda_0), & \text{for } \omega_{itl} = 0 \end{cases}, \\
 \omega_{itl} &\sim \text{Bernoulli}(p_\omega), \\
 d_{itl} &\sim \text{Unif}(0, 600), \\
 z_{itl} &\sim \text{Bernoulli}(\psi_{it}), \\
 \epsilon_{itl} &\sim \text{Bernoulli}(0.5), \\
 \text{logit}(\boldsymbol{\psi}) &= \mathbf{X}_\psi \boldsymbol{\beta}_\psi, \boldsymbol{\beta}_\psi \sim \mathcal{N}(\mathbf{0}, 2.25\mathbf{I}), \\
 \log(\boldsymbol{\lambda}) &= \mathbf{X}_\lambda \boldsymbol{\beta}_\lambda, \boldsymbol{\beta}_\lambda \sim \mathcal{N}(\mathbf{0}, 10\mathbf{I}), \\
 \lambda_0 &\sim \text{Gamma}(1.78, 0.675), \\
 p_\omega &\sim \text{Uniform}(0, 1).
 \end{aligned}$$

We set the informative prior for  $\lambda_0$  so that the mean size of a non-lek group observations was 1.2 and resulted in a prior probability of approximately 0.95 that a non-lek observation contains fewer than 4 individuals. The variance of  $\lambda_0$  implied the prior probability of a non-lek observation having less than 10 individuals was nearly 1.

## A.2 N-MIXTURE SUBMODEL

$$\begin{aligned}
F_{itlj} &\sim \text{Binomial}(N_{itl}^G, p) \text{ for } j = 1, \dots, J_{itl} \\
N_{itl}^G &\sim \text{Poisson}(\exp(\mathbf{w}'_{it}\boldsymbol{\eta})) \text{ for } l = 1, \dots, L_{it}^G, \\
\boldsymbol{\eta} &\sim \mathcal{N}(\mathbf{0}, 100\mathbf{I}), \\
p &\sim \text{Uniform}(0, 1).
\end{aligned}$$

## A.3 SPATIO-TEMPORAL TOBIT MODEL

$$\begin{aligned}
y_{it} &= \begin{cases} \zeta_{it}, & \text{for } \zeta_{it} > 0 \\ 0, & \text{for } \zeta_{it} \leq 0 \end{cases}, \\
\zeta_t &\sim \mathcal{N}(\boldsymbol{\xi}_t, \sigma_d^2 \mathbf{R}_d(\phi)), \\
\boldsymbol{\xi}_t &\sim \mathcal{N}((\boldsymbol{\xi}_{t-1}, \mathbf{W}_{t-1}) \boldsymbol{\alpha}, \text{Block-Diagonal}(\sigma_\tau^{2,A} \mathbf{I}_{n^A}, \sigma_\tau^{2,G} \mathbf{I}_{n^G})), \\
\boldsymbol{\xi}_0 &= \mathbf{X}_0 \boldsymbol{\gamma}, \\
\boldsymbol{\gamma} &\sim \mathcal{N}(\mathbf{0}, 100\mathbf{I}), \\
\alpha_j &\sim \text{Uniform}(-1, 1) \text{ for } j \in 1, 2 \\
\sigma_d^2 &\sim \mathcal{IG}(0.01, 100), \\
\sigma_\tau^{2,A} &\sim \mathcal{IG}(0.01, 100), \\
\sigma_\tau^{2,G} &\sim \mathcal{IG}(0.01, 100), \\
\phi &\sim \text{Discrete-Uniform}(1, 1001, 2001, \dots, 99001).
\end{aligned}$$

## B IMPLEMENTATION

We set  $\nu_d = 600$  which results in an approximate survey region of  $S = 2 \times 2 \times 15 \times 0.6 = 36 \text{ km}^2$  per survey block. We augmented our dataset to allow for  $M = 20$  groups per survey region. Both  $\nu_d$  and  $M$  were adequately large to accommodate uncertainty in the maximum detection distance and true number of LEPC groups in the sample population of each survey region (Royle et al., 2009). Both  $\nu_d$  and  $M$  can be set larger with no inferential impact on density but will increase computational burden because of the expanded parameter space.

The first-stage algorithm targeted samples from the joint distribution of the ADSM and N-mixture submodel with standard independent Metropolis-within-Gibbs samplers. The full-conditional distributions of the parameters  $\boldsymbol{\beta}_\lambda, \boldsymbol{\beta}_\rho, \mathbf{N}^{A,u}, \mathbf{d}^u, \boldsymbol{\epsilon}^u$ , and  $\mathbf{N}^G$  were non-tractable, thus we used a Metropolis-Hastings algorithm. To improve mixing, we updated the elements of each vector-valued parameter individually. We used normal random walk proposals for  $\boldsymbol{\beta}_\lambda, \boldsymbol{\beta}_\rho$ , and  $\boldsymbol{\eta}$ , and tuned the proposals such that acceptance rates varied between 20-40%. Proposals for  $\mathbf{N}^{A,u}, \mathbf{z}^u, \mathbf{d}^u, \boldsymbol{\epsilon}^u$ , and  $\mathbf{N}^G$  were generated from their prior distributions. The full-conditional distributions of  $\boldsymbol{\omega}, p_\omega, \mathbf{z}^u$ , and  $p$  were tractable, and we sampled directly from them using Gibbs updates. We obtained samples of  $\boldsymbol{\beta}_\psi$  using Pólya-Gamma data augmentation (Polson et al., 2013). We also considered Pólya-Gamma and Albert-Chib (Albert and Chib, 1993) data augmentation strategies for the linear predictor  $\boldsymbol{\beta}_\rho$  but found neither improved sampling efficiency.

The second-stage MCMC algorithm melded the submodel density samples  $y_{it}^A$  and  $y_{it}^G$  into the joint response spatial-temporal tobit model (STTM). Keeping notation general, we suppress the superscripts  $A$  and  $G$ , and let  $\mathcal{M}$  denote a generic submodel (in our case either the ADSM or N-mixture submodel). To meld the density samples, we drew a sub-sample of  $y_{it}$  from  $[y_{it}^{(\star)}, \cdot]_{\mathcal{M}}$ , denoted by  $y_{it}^{(\star)}$ , from the first-stage randomly with replacement, and the Metropolis-Hastings ratio was

$$\frac{[y_{it}^{(\star)} | \cdot]_{\text{STTM}}}{[y_{it}^{(k-1)} | \cdot]_{\text{STTM}}} \quad (1)$$

where  $[y_{it}^{(\star)} | \cdot]_{\text{STTM}}$  is the conditional distribution of  $y_{it}^{(\star)}$  given the current value of all other parameters in the STTM. Letting  $\theta^{(k)}$  denote the value of parameter  $\theta$  at iteration  $k$ , we have that for  $y_{it}^{(\star)} = 0$ ,

$$[y_{it}^{(\star)} | \cdot]_{\text{STTM}} = \mathcal{P}(\zeta_{it} \leq 0 | \zeta_{-it}^{(k-1)}, \boldsymbol{\xi}_t^{(k-1)}, \sigma_d^{2,(k-1)}, \phi^{(k-1)}) = \Phi(0 | \tilde{\mu}^{(k-1)}, \tilde{\sigma}^{2,(k-1)}), \quad (2)$$

and if  $y_{it}^{(\star)} > 0$ , then

$$[y_{it}^{(\star)} | \cdot]_{\text{STTM}} = \mathcal{N}(\tilde{\mu}^{(k-1)}, \tilde{\sigma}^{2,(k-1)}), \quad (3)$$

where  $\Phi$  is the cumulative distribution function of the standard normal distribution and

$$\tilde{\mu}^{(k-1)} = \xi_{it}^{(k-1)} + \mathbf{r}_{d,i-i}(\phi^{(k-1)}) (\mathbf{R}_{d,-i-i}(\phi^{(k-1)}))^{-1} (\boldsymbol{\zeta}_{-it}^{(k-1)} - \boldsymbol{\xi}_{-it}^{(k-1)}), \quad (4)$$

$$\tilde{\sigma}^{2,(k-1)} = \sigma_d^{2,(k-1)} \left( r_{d,ii}(\phi^{(k-1)}) - \mathbf{r}_{d,i-i}(\phi^{(k-1)}) (\mathbf{R}_{d,-i-i}(\phi^{(k-1)}))^{-1} \mathbf{r}_{d,-ii}(\phi^{(k-1)}) \right). \quad (5)$$

The acceptance rates of our Metropolis-Hastings algorithms for  $y_{it}^A$  and  $y_{it}^G$  were 30% and 49%, respectively.

For  $y_{it} > 0$ ,  $\zeta_{it}$  is known and  $\zeta_{it} = y_{it}$ , but for  $y_{it} = 0$ ,  $\zeta_{it}$  is latent and must be sampled from its full-conditional distribution. We sampled the vector of latent quantities  $\boldsymbol{\zeta}_t^u$  with a Gibbs update because its full-conditional distribution is multivariate normal truncated at 0. The full-conditional distributions of  $\boldsymbol{\xi}_t$  and  $\boldsymbol{\gamma}$  are multivariate normal and were sampled from using Gibbs updates. Likewise, the full-conditional distribution for  $\boldsymbol{\alpha}$  was multivariate normal truncated between  $-1$  and  $1$ . We also used Gibbs updates for the variance parameters  $\sigma_\tau^{2,A}$ ,  $\sigma_\tau^{2,G}$ , and  $\sigma_d^2$  which have inverse-gamma full-conditional distributions. A Metropolis-Hastings algorithm was employed for updating  $\phi$ . We precalculated the exponentially decaying distance correlation matrices,  $\mathbf{R}(\phi)$ , associated with each support value of  $\phi$  to improve computation.

## C COVARIATES

We selected a parsimonious suite of covariates previously shown to be associated with LEPC demography, occupancy, and abundance that quantify differences in landcover, habitat patch size, anthropogenic disturbance, and climatic stochasticity. Table 1 provides a description of each covariate, indicates its source, and where it was used. All covariates were measured at the  $15 \times 15$  km survey block resolution except for Palmer Drought Severity Index (PDSI) which was extracted from the nine Kansas climate divisions. All continuous covariates except for PDSI were standardized to have mean 0 and variance 1. To derive covariate values for the ground sites, we calculated a weighted average of the survey block covariate values based on the percentage of area the ground survey region included each block. Only PDSI was temporally indexed. All other covariates were static and

measured in 2012.

Table 1: Covariates available at following links:

WEST (field-collected data from WEST aerial surveys),  
 NLCD (<https://www.mrlc.gov/data/references/national-land-cover-database-2011-nlcd2011>),  
 NRCS (<https://www.nrcs.usda.gov/wps/portal/nrcs/site/national/home/>),  
 USDA (United States Department of Agriculture (USDA) (2014)),  
 NOAA (<https://www.ncei.noaa.gov/access/monitoring/historical-palmers/maps>).

| Name                 | Description                                                            | Source | Design Matrices                                                      |
|----------------------|------------------------------------------------------------------------|--------|----------------------------------------------------------------------|
| Ecoregion            | Ecoregion identifier (1 = SSPR, 2 = MGPR, 3 = SGPR)                    | WEST   | $\mathbf{X}_\lambda, \mathbf{X}_\psi, \mathbf{X}_0, \mathbf{X}_\rho$ |
| Development          | Percentage of area (%) with anthropogenic development.                 | NLCD   | $\mathbf{X}_\lambda, \mathbf{X}_\psi, \mathbf{X}_0$                  |
| CRP                  | Percentage of area (%) enrolled in the Conservation Reserve Program.   | USDA   | $\mathbf{X}_\lambda, \mathbf{X}_\psi, \mathbf{X}_0$                  |
| Grassland patch size | Average size (km <sup>2</sup> ) of grassland landcover patches.        | NLCD   | $\mathbf{X}_\lambda, \mathbf{X}_\psi, \mathbf{X}_0$                  |
| Shrubland            | Percentage of area (%) dominated by shrubs, including trees <5 m tall. | NLCD   | $\mathbf{X}_\lambda, \mathbf{X}_\psi, \mathbf{X}_0$                  |
| Woodland             | Percentage of area (%) with tree canopy cover >1%.                     | NRCS   | $\mathbf{X}_\lambda, \mathbf{X}_\psi, \mathbf{X}_0$                  |
| PDSI                 | Palmer Drought Severity Index averaged over March, April, and May.     | NOAA   | $\mathbf{X}_\lambda, \mathbf{X}_\psi, \mathbf{W}_t$                  |

## D POSTERIOR INFERENCE FOR COVARIATE ASSOCIATIONS

Posterior mean LEPC densities were highest in the SGPR ecoregion and lowest in the SSPR (Table 2). The MGPR ecoregion had interemediate LEPC densities. LEPC densities were lower in regions with a higher percentage of anthropogenic disturbance and tree canopy cover. LEPC density was positively associated with the percentage of area enrolled in the Conservation Reserve Program (CRP), percentage of area dominated by shrubs, and average size of grassland landcover patches. The autoregressive parameter suggested strong positive temporal dependence in LEPC densities. On average, LEPC densities were lower in drier years.

Table 2: Posterior means and credible interval for regression coefficients  $\gamma$  and  $\alpha$ .

| Covariate                | Parameter  | Posterior Mean | Credible Interval (90%) |
|--------------------------|------------|----------------|-------------------------|
| SSPR                     | $\gamma_0$ | 0.026          | (-0.24, 0.30)           |
| MGPR                     | $\gamma_1$ | 0.33           | (0.12, 60)              |
| SGPR                     | $\gamma_2$ | 0.55           | (0.38, 0.73)            |
| Development              | $\gamma_3$ | -0.22          | (-0.29, -0.16)          |
| CRP                      | $\gamma_4$ | 0.12           | (0.081, 0.16)           |
| Grassland patch size     | $\gamma_5$ | 0.42           | (0.31, 0.55)            |
| Shrubland                | $\gamma_6$ | 0.28           | (0.17, 0.39)            |
| Woodland                 | $\gamma_7$ | -0.12          | (-0.20, -0.05)          |
| Autoregressive parameter | $\alpha_0$ | 0.99           | (0.98, 1)               |
| PDSI                     | $\alpha_1$ | 0.013          | (0.0, 0.026)            |

## References

Albert, J. H. and Chib, S. (1993). Bayesian analysis of binary and polychotomous response data. *Journal of the American Statistical Association*, 88(422):669–679.

- Polson, N. G., Scott, J. G., and Windle, J. (2013). Bayesian inference for logistic models using Pólya–Gamma latent variables. *Journal of the American Statistical Association*, 108(504):1339–1349.
- Royle, J. A., Karanth, K. U., Gopalaswamy, A. M., and Kumar, N. S. (2009). Bayesian inference in camera trapping studies for a class of spatial capture–recapture models. *Ecology*, 90(11):3233–3244.
- United States Department of Agriculture (USDA) (2014). Common Land Unit geospatial data. Memorandum of understanding between the USDA the Western Association of Fish and Wildlife Agencies, signed 21 February 2014.
